# Supplementary material for: Hydra: A System for Large Multi-Model Deep Learning
Source: arXiv:2110.08633 source file (2022-08-03)
Supplement: Supplementary file 1 [file supplementary_material.pdf]

# Supplementary Materials for Model-Parallel Task Parallelism for Efficient Multi-Large-Model Deep Learning

**Anonymous Author(s)**
Affiliation
Address
email

# A Appendix

## A.1 HYDRA API Usage

HYDRA's API is designed to be accessible and easy to integrate into existing codebases. The user instantiates their model architectures using standard PyTorch definitions, then provides the model to HYDRA's task wrapper along with a name (used for identification in user-facing logging), a loss function, a PyTorch-defined dataloader for data processing, a learning rate, and the number of epochs to run.

```
model = PyTorchModel()
dataloader = get_dataloader()
task = hydra.ModelTask("name", model, loss_fn, dataloader, 1e-4, 5)
```

Once several models are defined in this fashion, the user can provide a list of tasks to our automatic orchestrator. The user first specifies to the orchestrator how much of a buffer space to retain for double-buffering, then runs the automatic partitioner before making the final call for the training loop to begin.

```
orchestra = ModelOrchestrator([task_0, task_1, task_2, task_3])
orchestra.buffer = 15000 # about 1GB
orchestra.generate()
orchestra.train_models()
```

In general, HYDRA can be integrated into a codebase with only 10-15 additional lines of code and minimal configuration.

## A.2 MILP Formulation of Scheduler and Evaluations

We now present our formulation of the batched multi-large-model scheduling workload with the objective of minimizing end-to-end runtimes.

The scheduling problem is as follows. When a device (GPU) becomes available, a shard unit must be selected from one the model's queues to be placed upon that device. Shard units become *eligible* for scheduling if they have no pending dependencies, i.e., they are at the front of their queue and no other shard unit of that same model is still running on another device. The Scheduler's job is to pick a shard unit from the set of eligible shard units. Double-buffered training is already factored into this formulation: the Scheduler is actually picking shard units for double-buffering, and they get promoted from the buffer to compute.

Submitted to 36th Conference on Neural Information Processing Systems (NeurIPS 2022). Do not distribute.

Table 1: Notation for our scheduling formalization.

| Symbol | Description |
|---|---|
| $T$ | List of models specified by the user to be trained |
| $P$ | List of devices (GPUs) available for training. |
| $M_i \in \mathbb{Z}^+$ | $M_i$ is the total number of shard units for model $T_i \in T$. Note that this covers all mini-batches (and potentially epochs). |
| $S_i \in \mathbb{R}^{M_i}$ | $S_i$ is a variable-length list of shard unit runtimes for model $T_i$. The runtime of shard unit $j$ is denoted as $S_{i,j}$. |
| $X_i \in \mathbb{R}^{\lvert P\rvert \times \lvert M_i\rvert}$ | $X_i$ is a variable-shape matrix of start times of shard units of model $T_i$ across workers. The start time of shard unit $j$ on worker $p$ is denoted as $X_{i,p,j}$. Note that this linear ordering covers not just the model's forward and backward passes but also ordering across mini-batches (and potentially epochs). |
| $Y_i \in \{0,1\}^{\lvert \mathrm{P}\rvert \times \mathrm{L} \times \mathrm{L}}$ | $L$ is the total number of shard units across all models, i.e., $L = \sum_i M_i$, indexed cumulatively by the index of model $i$ and its shard unit $j$ (denoted $i\_j$). $Y_{p,i\_j,i'\_j'} = 1 \Leftrightarrow X_{i,p,j} < X_{i',p,j'}$. |
| $U$ | An extremely large value used to enforce boolean logic. |

All shard unit runtimes are given as input. Recall from Section 2 from the main paper that the partitioner records this data during its pilot run. We now present the formal scheduling problem as an MILP. Table 1 explains our notation.

$$\texttt{Objective:} \quad \min_{X,Y} C \tag{1}$$

`Constraints:`

$$\begin{aligned}
&\forall t, t' \in [1, \ldots, |T|] \quad \forall p, p' \in P \\
&(a)\ \forall j \in [2, \ldots, M_t]\ X_{t,p,j} \geq X_{t,p',j-1} + S_{t,j-1} \\
&(b)\ \forall j \in [1, \ldots, M_t] \quad \forall j' \in [1, \ldots, M_{t'}] \\
&\quad X_{t,p,j} \geq X_{t',p,j'} + S_{t',j'} - (U \times Y_{p,t_j,t'_j'}) \\
&(c)\ \forall j \in [1, \ldots, M_t] \quad \forall j' \in [1, \ldots, M_{t'}] \\
&\quad X_{t,p,j} \leq X_{t',p,j'} - S_{t,j} + (U \times (1 - Y_{p,t_j,t'_j'})) \\
&(d)\ \forall j \in [1, \ldots, M_t] \\
&\quad X_{t,p,j} \geq 0 \\
&(e)\ \forall j \in [1, \ldots, M_t] \\
&\quad C \geq X_{t,p,j} + S_{t,j}
\end{aligned} \tag{2}$$

The objective is to pick a shard unit that can minimize makespan (completion time of the whole workload at this granularity). Constraints (a) simply enforce the *sequential ordering of shard units* within a model. Note that this set per model here is unified within a mini-batch, across mini-batches within an epoch, and potentially across epochs too–they are all sequentially dependent. Constraints (b) and (c) enforce *model training isolation*, i.e., only one shard unit can run on a device at a time. Constraints (d) is just non-negativity of start times, while Constraints (e) define the makespan.

Using a MILP solver such as Gurobi [1] enables us to produce an "optimal" schedule in this context. But the above task is a variant of a general job-shop scheduling problem described in [4], and it is known to be NP-complete. Given that the number of shard units can span thousands to tens of millions, solving it optimally will likely be impractically slow. This motivates our design of Sharded-LRTF, an approximate greedy algorithm that maximizes utilization by pushing all tasks to complete at the same time.

**Algorithm 1** The Sharded-LRTF scheduling algorithm.

**Struct {**
  Remaining epochs $e$
  Minibatches per epoch $b$
  Remaining minibatches in current epoch $ce$
  Minibatch training time $t$
  Remaining train time in current minibatch $cm$
}
**Input:** Idle Models $[M]$
**Output:** Model $MaxModel$
$MaxTrainTime = 0$
**for** Index $i$, Model $m$ in $[M]$ **do**
  $ModelTrainTime$ =$((m_e - 1) \times m_b + m_{ce} - 1) \times m_t + m_{cm}$
  **if** $ModelTrainTime > MaxTrainTime$ **then**
    $MaxTrainTime = ModelTrainTime$
    $MaxModel = m$
  **end if**
**end for**

Algorithm 1 describes the algorithm in depth, and we provide evaluations on simulated workloads against a random selection baseline and Gurobi-Optimal with a 100s timeout in Figure 1. Note that Gurobi-Optimal often seems to fail to converge within the given time-budget, further illustrating its impracticality as a scheduler within an ongoing multi-large-model workload.

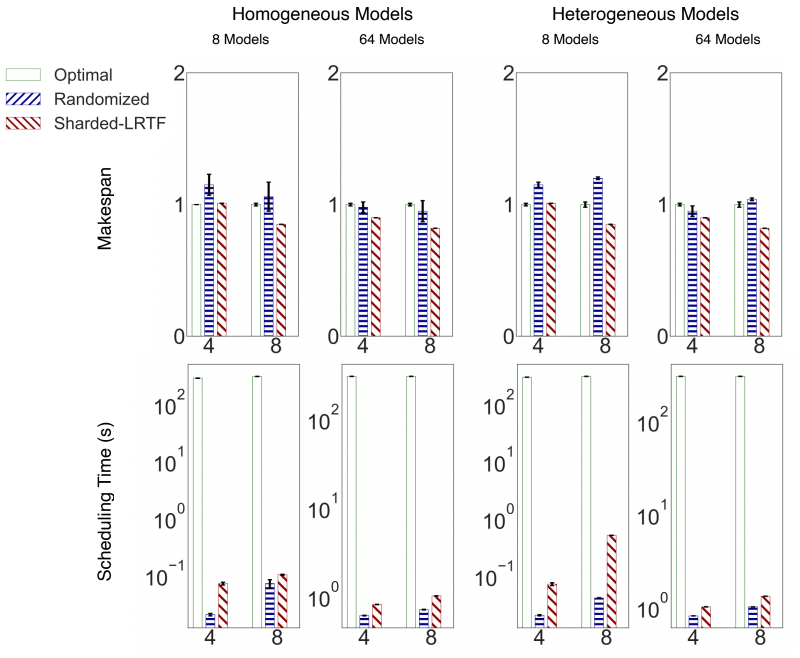


Figure 1: Comparison of various scheduling algorithms. Makespans are normalized to Optimal.

Our current selection procedure runs in linear time to find the task with the longest expected runtime. Using an alternate data structure could enable constant time selection, but the benefits would be marginal.

### A.3 Grid Search Results

We report on the perplexity results produced by each hyperparameter configuration from our grid search experiments. The results are identical across training techniques (model parallelism, ZeRO-3, HYDRA, and GPipe). Training is run with a context size of 512 and the SGD optimizer.

| Learning Rate | Batch Size | Test Perplexity | Validation Perplexity |
|---|---|---|---|
| 0.0003 | 8 | 15.17 | 15.69 |
| 0.0003 | 16 | 15.34 | 15.87 |
| 0.0001 | 8 | 15.50 | 16.04 |
| 0.0001 | 16 | 15.23 | 15.75 |
| 0.00006 | 8 | 15.33 | 15.84 |
| 0.00006 | 16 | 15.34 | 15.87 |
| 0.00005 | 8 | 15.41 | 15.95 |
| 0.00005 | 16 | 15.49 | 16.02 |
| 0.00002 | 8 | 15.36 | 15.94 |
| 0.00002 | 16 | 15.50 | 16.02 |
| 0.00001 | 8 | 15.50 | 16.03 |
| 0.00001 | 16 | 15.54 | 16.07 |

Table 2: Fine-tuned GPT-2 [3] perplexity scores for language modeling on the WikiText-2 [2] dataset.

## References

[1] LLC Gurobi Optimization. Gurobi Optimizer Reference Manual. 2021.

[2] Stephen Merity, Caiming Xiong, James Bradbury, and Richard Socher. Pointer sentinel mixture models. *CoRR*, abs/1609.07843, 2016.

[3] Alec Radford et al. Language models are unsupervised multitask learners. *OpenAI blog*, 1(8):9, 2019.

[4] J.D. Ullman. NP-Complete Scheduling Problems. *Journal of Computer , System Sciences.*, 10(3):384–393, June 1975.
